# Supplementary material for: Spin-Reorientation-Driven Linear Magnetoelectric Effect in Topological Antiferromagnet Cu$_3$TeO$_6$
Source: arXiv:2211.08902 source file (2024-02-28)
Supplement: Supplementary file 1 [file Supplement.pdf]

# Linear Magnetoelectric Effect in Topological Antiferromagnet $\text{Cu}_3\text{TeO}_6$ : Supplemental material

Virna Kisiček,<sup>1,2,\*</sup> Damir Dominko,<sup>1</sup> Matija Čulo,<sup>1</sup> Marko Kuveždić,<sup>3</sup> Željko Rapljenović,<sup>1</sup>  
Martina Dragičević,<sup>1</sup> Helmuth Berger,<sup>4</sup> Mirta Herak,<sup>1,†</sup> and Tomislav Ivek<sup>1</sup>

<sup>1</sup>*Institute of Physics, Bijenička cesta 46, 10 000 Zagreb, Croatia*

<sup>2</sup>*Faculty of Physics, University of Rijeka,  
Ul. Radmile Matejčić 2, 51000 Rijeka, Croatia*

<sup>3</sup>*Department of Physics, Faculty of Science,  
University of Zagreb, Bijenička cesta 32, 10 000 Zagreb, Croatia*

<sup>4</sup>*Institute of Physics, Ecole Polytechnique Fédérale de Lausanne (EPFL), CH-1015 Lausanne, Switzerland*

(Dated: November 16, 2022)

## I. RESULTS OF SIMULATIONS OF MAGNETIC STRUCTURE IN GROUND STATE AND APPLIED MAGNETIC FIELD FOR $J_1 - J_9$ MODEL WITH DZIALOSHINSKII-MORIYA INTERACTION

To simulate the magnetic ground state and magnetic-field induced states in  $\text{Cu}_3\text{TeO}_6$ , we have taken into account only first-nearest-neighbor interactions  $J_1$  and ninth-nearest-neighbor interactions  $J_9$ , which connect the spins being 3.18 Å and 6.21 Å apart, respectively. The magnetic unit cell consists of 12 magnetically inequivalent copper atoms which we use as a basic unit in our calculations. In the left panel of Fig. S1 we plot all the interactions  $J_1$  and  $J_9$  that connect spins in one magnetic cell to other spins. Each spin interacts through  $J_1$  with four magnetically inequivalent spins and through  $J_9$  with four other spins which are each magnetically equivalent to one of  $J_1$  spins. E.g. spin 1 is connected through  $J_1$  to the first neighboring spins 2, 6, 8 and 10, and through  $J_9$  to the ninth-neighboring spins 2, 6, 8 and 10. Therefore, when these interactions are mapped onto single magnetic unit cell, the effective magnetic lattice shown in the right panel of Fig. S1 is obtained. In our model we assume that Dzyaloshinskii-Moriya [1] is present only between the spins coupled by  $J_1$ . If this anisotropy was not present there would be no difference between the model with isotropic  $J_1$  and  $J_9$  and the model with only  $J_1$  present with magnitude equal to the sum of  $J_1$  and  $J_9$  of the first model.

The calculated ground state for the  $J_1 - J_9$  model [2] with Dzyaloshinskii-Moriya interaction

---

\* [vkisicek@ifs.hr](mailto:vkisicek@ifs.hr)

† [mirta@ifs.hr](mailto:mirta@ifs.hr)

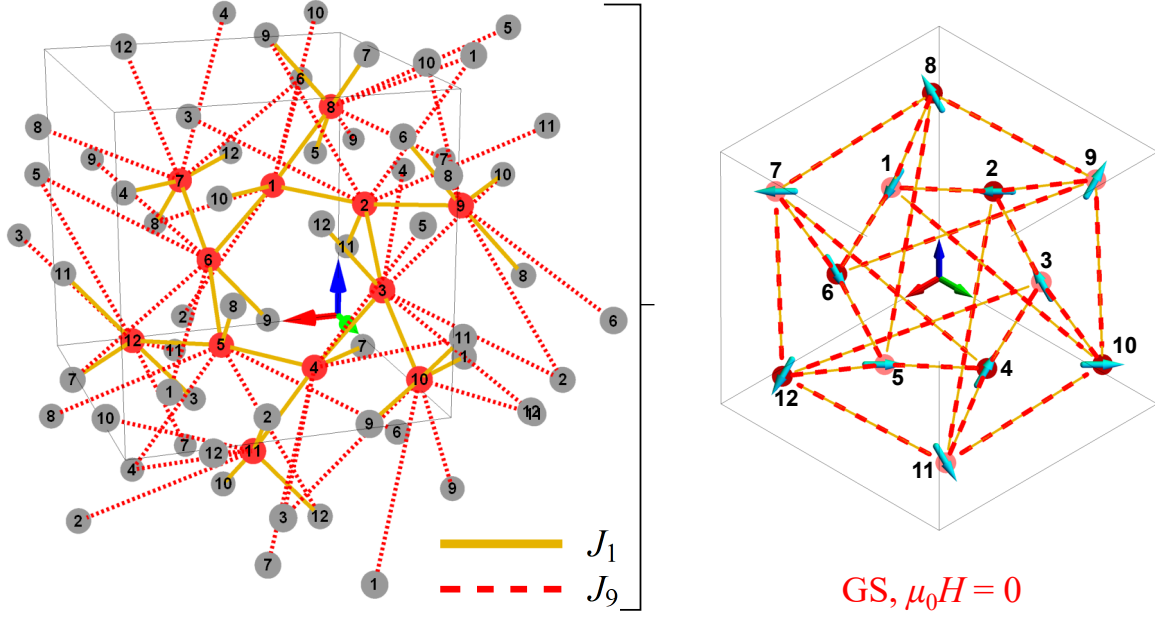

**FIG. S1:** Left panel: atoms belonging to one primitive magnetic unit cell are shown as red spheres. All the gray spheres belong to other magnetic cells. There are 12 magnetically inequivalent coppers in crystal unit cell, where each carries a label from 1-12. First-nearest neighbor interaction  $J_1$  between the coppers that are  $3.12 \text{ \AA}$  apart is shown in solid gold line. Ninth-nearest-neighbor interaction  $J_9$  is shown by dashed red line. For the sake of clarity only interactions which involve spins in one magnetic cell (red) are shown, as well as only atoms which participate in those interactions. When these interactions are mapped onto magnetic unit cell, the effective magnetic lattice shown in the right panel is obtained. Right panel: Antiferromagnetic ground state of  $\text{Cu}_3\text{TeO}_6$ . The dark and light red spheres represent the major up and down component of the spins which are (anti)parallel to the space diagonal  $[111]$  in this domain. The blue arrows represent the canted component ( $30\times$  magnified) induced by the Dzyaloshinskii-Moriya interaction. The canted component is perpendicular to the main component. The numbers mark the twelve magnetically inequivalent copper atoms to be compared to the red magnetic unit cell on the left. Gold solid line and dashed red line represent the  $J_1$  and  $J_9$  interactions, respectively.

between first nearest neighboring spins is 8 times degenerate with spins predominantly being predominantly oriented in the direction of one of the space diagonals of the cubic unit cell (see left panel in Fig. S1). The choice of parameters is  $J_1/k_B = 55 \text{ K}$ ,  $J_9/k_B = 55 \text{ K}$  and  $D = 0.1J_1$ , as explained in the main text. The 8 domains are shown in Fig. S2. There are four different orientations of the domains where the two domains with same orientation are connected by time inversion  $1'$ . The small canting induced by DMI which gives the angle between the nearest neighboring spins of  $178.85^\circ$ . The Dzyaloshinskii-Moriya interaction is responsible for the anisotropy

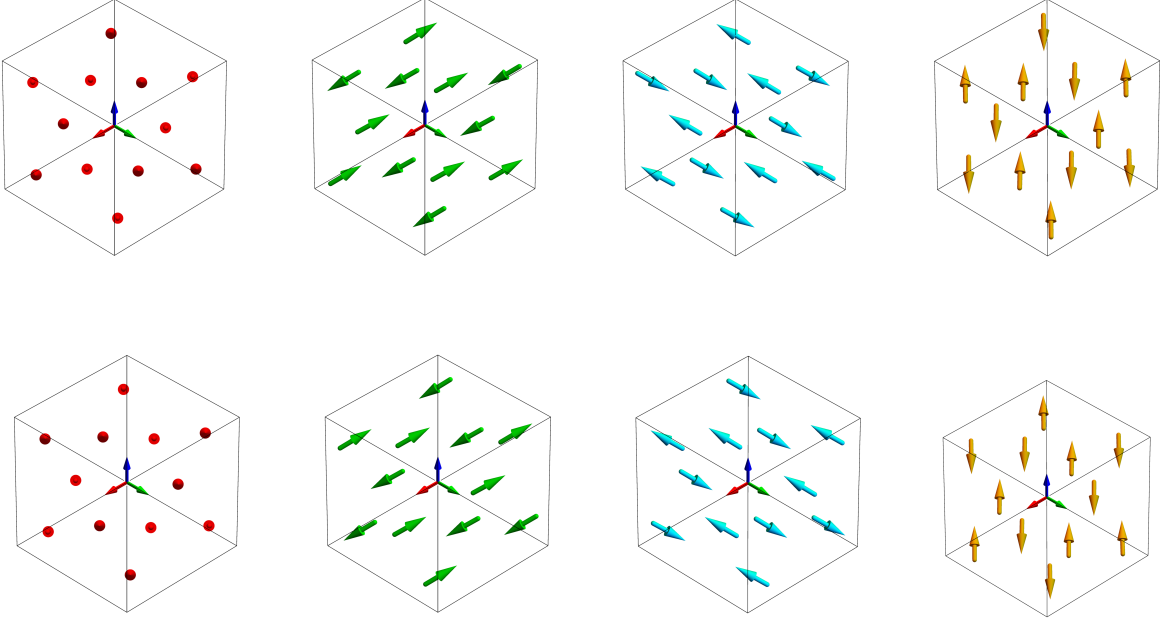

**FIG. S2:** 8 AFM domains calculated as the ground state of the Hamiltonian (1) in the main text.

Domains in bottom panels have equivalent orientations as the corresponding ones in the top panel, but with opposite AFM easy axis directions. The domains with same color can be obtained one from the other by applying the time inversion symmetry element  $1'$ . Red, green and blue arrows in the corner denote the  $(a, b, c)$  crystal axes of the cubic crystal system.

which determines the orientation of the spins in the ground state. The 8 resulting AFM domains are plotted in Fig. S2. The magnetic point group symmetry of the obtained ground state is  $\bar{3}'$ , in complete agreement with the experimentally determined magnetic ground state structure [3]. The calculated ground state preserves the  $\bar{1}'$  symmetry.

The magnetic structure was determined for finite magnetic field applied along several different directions. We find that already in small field  $H \gtrsim 0.5$  T the spins fully reorient to another direction, where spin reorientation is driven by total energy minimization in applied magnetic field, equivalent to the spin-flop phenomenon in uniaxial AFMs. In our calculation a specific domain ground state was selected as a starting point and then the field was slowly increased and the free energy minimum was calculated by taking the previous result as a starting point. We summarize the results in table S1 for several special crystallographic directions (with respect to cubic crystallographic system). The number of different domains reduces in applied field. For  $\mathbf{H} \parallel [001]$  only two orientational domains i.e. 4 AFM domains are present with spin axis in either  $[110]$  or  $[\bar{1}10]$  and equivalent directions. The similar result is obtained for  $\mathbf{H} \parallel [010]$ , while for  $\mathbf{H} \parallel [111]$  six AFM

| Domain            | $H \parallel [001]$ | $H \parallel [111]$                           | $H \parallel [010]$ |
|-------------------|---------------------|-----------------------------------------------|---------------------|
| [111]             | [110]               | $[11\bar{2}]$ , $[\bar{2}11]$ , $[1\bar{2}1]$ | [101]               |
| $\bar{1}\bar{1}1$ | $\bar{1}\bar{1}0$   | $\bar{2}11$                                   | $\bar{1}01$         |
| $1\bar{1}\bar{1}$ | $\bar{1}\bar{1}0$   | $1\bar{2}1$                                   | [101]               |
| $11\bar{1}$       | [110]               | $11\bar{2}$                                   | $\bar{1}01$         |

**TABLE S1:** The direction of the spin axis in applied field for each domain and different field directions. The direction is achieved in fields higher than critical, in lower fields, the spin axis gain component along these directions.

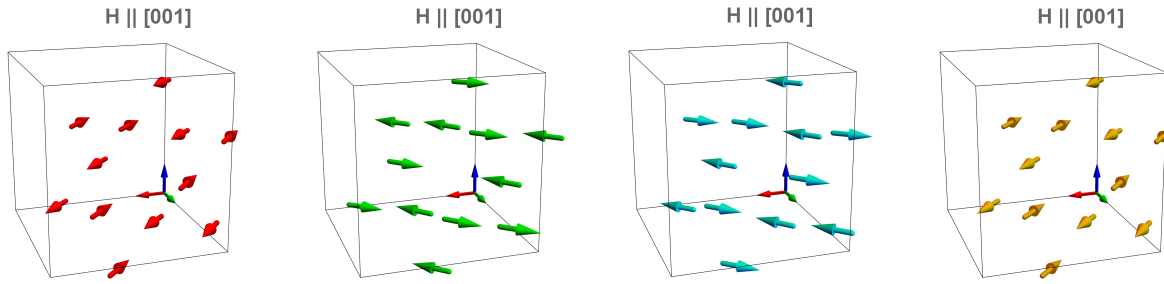

**FIG. S3:** AFM domains calculated for  $H = 5$  T applied in the direction [001] (blue arrow). The result for each of 4 different orientational AFM moments is plotted using same colors as in Fig. S2. Only 2 orientational domains can be distinguished both with magnetic point group symmetry  $m \perp H$ . Magnetic field reduces the degeneracy of the total number of possible AFM domains to 4.

domains are found.

The magnetic structure calculated for  $\mathbf{H} \parallel [001]$  is shown in Fig. S3. The magnetic point group symmetry of the calculated structure is  $m \perp [001]$ . The magnetic structure calculated for  $H \parallel [010]$  is shown in Fig. S4. The magnetic point group symmetry of the calculated structure is  $m \perp [010]$ . We can conclude that for  $\mathbf{H}$  along one of the cubic crystal axes the magnetic point group symmetry is  $m$  with  $m \perp H$ .

Magnetization for separate domains was calculated for two field directions used in experiment. The result for  $\mathbf{H} \parallel [001]$  is shown in Fig. S5. All domains are equivalent for this field direction and give the same bulk magnetization. Only orientationally different domains were considered since domains with the same easy axis cannot be distinguished in bulk magnetization experiment.

The situation is different for  $\mathbf{H} \parallel [111]$  where the domain D1 (which contains two domains with easy axis along [111]) shows behaviour typical for uniaxial AFM where spin-flop can be observed at critical field  $\mu_0 H_{SF} \approx 1$  T. For other three (six) domains magnetization is linear in applied field.

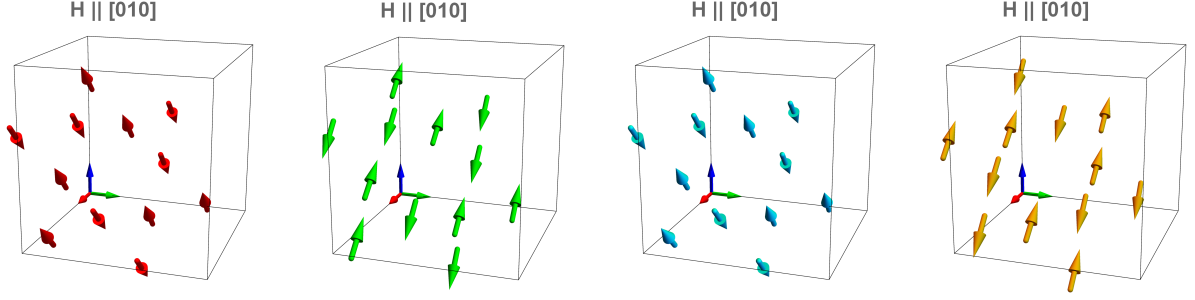

**FIG. S4:** AFM domains calculated for  $H = 5$  T applied in the direction  $[010]$  (green arrow). The result for each of 4 different orientational AFM moments is plotted using the same colors as in Fig. S2. Only 2 orientational domains can be distinguished both with magnetic point group symmetry  $m \perp H$ . Magnetic field reduces the degeneracy of the total number of possible AFM domains to 4.

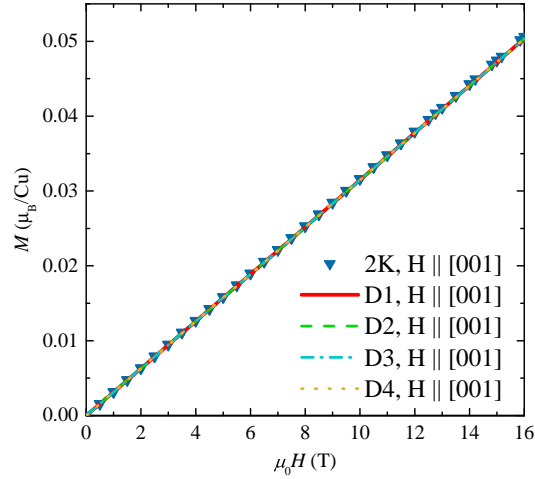

**FIG. S5:** Comparison of magnetization curves calculated for  $\mathbf{H} \parallel [001]$ , for separate orientational domains D1, D2, D3 and D4 with experiment. While each orientation allows two domains connected by  $1'$ , these cannot be distinguished in bulk magnetization measurements.

This is captured in the left panel of Fig. S6, while in the right panel a small misorientation of the sample is simulated by offsetting the direction of the magnetic field by  $1^\circ$  from  $[111]$  direction.

In the main text we show the total magnetization as the average of four distinguishable domains under assumption that all domains are equally populated. As can be seen from Fig. S5, even if that assumption is not satisfied, it would not be observed in experiment for  $\mathbf{H} \parallel [001]$  since all domains give the same contribution to the measured  $M$ . For  $\mathbf{H} \parallel [111]$  it would be possible, in principle, to distinguish the domain D1 from the rest, however, even a small misorientation of the sample might mask the effect of nonequivalent domains.

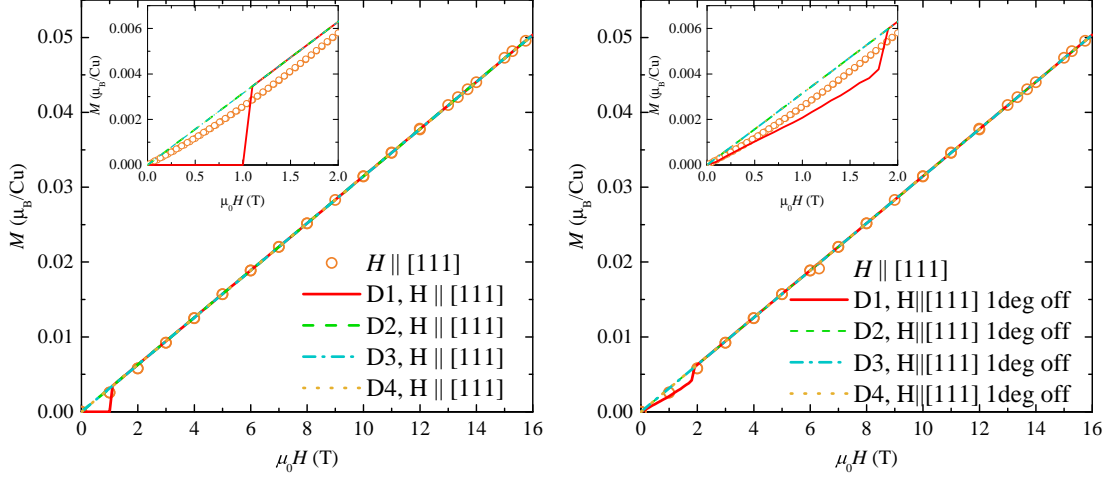

**FIG. S6:** Comparison of magnetization curves calculated for separate orientational domains, D1, D2, D3 and D4 with experiment. Left panel:  $\mathbf{H} \parallel [111]$ . Right panel:  $\mathbf{H}$  is offset by  $1^\circ$  from  $[111]$  direction.

## II. MAGNETOELECTRIC TENSOR IN $\text{Cu}_3\text{TeO}_6$ BASED ON CALCULATIONS

Our calculations show that already in modest magnetic field  $H \gtrsim 0.5$  T spins fully reorient into different directions. For  $H \parallel [001]$  we obtain the point group symmetry  $m$  with  $m \perp [001]$  or rather  $m \perp \mathbf{H}$ . This symmetry also allows the magnetoelectric effect [4]. The magnetoelectric tensor is given by [4]

$$\boldsymbol{\alpha} = \begin{bmatrix} 0 & 0 & \alpha_{13} \\ 0 & 0 & \alpha_{23} \\ \alpha_{31} & \alpha_{32} & 0 \end{bmatrix}, \quad (\text{S1})$$

where  $X3 = [001]$ , or rather the axis  $X3 \parallel H$ . This tensor has no diagonal elements. For magnetic field  $H \parallel X3 = (0, 0, H)$  we obtain

$$P_1 = \alpha_{13}H \quad (\text{S2})$$

$$P_2 = \alpha_{23}H \quad (\text{S3})$$

$$P_3 = 0. \quad (\text{S4})$$

This, however is a result for just one of the domains. The other, perpendicular domain will have the tensor rotated by  $90^\circ$  around  $[001]$  axis giving the following

$$P_1 = \alpha_{23}H \quad (\text{S5})$$

$$P_2 = \alpha_{13}H \quad (\text{S6})$$

$$P_3 = 0. \quad (\text{S7})$$

The polarization measured along the axis  $X1 = [100]$  will thus depend on two tensor components. For  $\mathbf{H} \parallel [010]$  the symmetry is also  $m$ , but now  $m \perp [010]$  since the spins will reorient into direction  $[101]$  and equivalent (see table S1) in order to be perpendicular to the magnetic field. This gives the following tensor [4]

$$\boldsymbol{\alpha} = \begin{bmatrix} 0 & \alpha_{12} & 0 \\ \alpha_{21} & 0 & \alpha_{23} \\ 0 & \alpha_{32} & 0 \end{bmatrix}. \quad (\text{S8})$$

The resulting polarization components for  $H \parallel [010]$  for one of the domains are

$$P_1 \sim \alpha_{12}H \quad (\text{S9})$$

$$P_2 \sim 0 \quad (\text{S10})$$

$$P_3 \sim \alpha_{32}H, \quad (\text{S11})$$

while for the other orientational domain

$$P_1 \sim \alpha_{32}H \quad (\text{S12})$$

$$P_2 \sim 0 \quad (\text{S13})$$

$$P_3 \sim \alpha_{12}H. \quad (\text{S14})$$

Again the polarization measured along  $[100]$  will depend on two tensor components. However, if the population of domains is different for different applied field directions, the magnitude of polarization measured along the specific direction can in principle be different even for symmetrically equivalent field directions  $[010]$  and  $[001]$ , while in bulk magnetization measurements we would observe no difference. This can be understood if we take a look at the easy axis directions for different domains in applied field for  $\mathbf{H} \parallel [001]$  and  $\mathbf{H} \parallel [010]$ . For the sake of argument, we can assume that only orientationally different domains  $[111]$  and  $[11\bar{1}]$  are present in the ground state of the sample. For  $\mathbf{H} \parallel [001]$  these domains in our calculations collapse into the same domain with spin axis  $\parallel [110]$ . However, for  $\mathbf{H} \parallel [010]$ , they collapse in two orientationally different domains, with easy axis  $\parallel [101]$  and  $\parallel [\bar{1}01]$ . Thus, we can expect different measured polarization magnitude when the field is applied along these crystallographically equivalent directions. Furthermore, different samples could give different polarization magnitudes in comparison to what was observed in our experiment.

To summarize, the shape of the magnetoelectric tensor obtained for calculated spin reoriented configuration in applied magnetic field with point group symmetry  $m \perp \mathbf{H}$  is consistent with the

experiment where only off-diagonal elements are present. Different domain population can qualitatively explain the different magnitude of polarization measured along the same crystallographic direction for the two perpendicular, but symmetric field directions.

- 
- [1] I. Dzyaloshinsky, [Journal of Physics and Chemistry of Solids](#) **4**, 241 (1958); T. Moriya, [Phys. Rev.](#) **120**, 91 (1960).
  - [2] W. Yao, C. Li, L. Wang, S. Xue, Y. Dan, K. Iida, K. Kamazawa, K. Li, C. Fang, and Y. Li, [Nature Phys.](#) **14**, 1011–1015 (2018).
  - [3] M. Herak, H. Berger, M. Prester, M. Miljak, I. Živković, O. Milat, D. Drobac, S. Popović, and O. Zaharko, [Journal of Physics: Condensed Matter](#) **17**, 7667 (2005).
  - [4] R. E. Newnham, *Properties of Materials (Anisotropy, Symmetry, Structure)* (Oxford University Press, New York, USA, 2005).
